# Supplementary material for: SynLLM: A Comparative Analysis of Large Language Models for Medical Tabular Synthetic Data Generation via Prompt Engineering
Source: arXiv:2508.08529 source file (2025-08-11)
Supplement: Supplementary file 1 [file 80-Appendix.tex]

\appendix

\section*{Appendix: Supplementary Material}

\subsection*{Parallel Computing}
To optimize runtime and handle large-scale synthetic data generation, we employed parallel computing techniques across heterogeneous GPU nodes. Using GNU Parallel, we orchestrated concurrent model inference jobs, enabling the simultaneous evaluation of multiple language models and prompt variants. Each job was distributed over separate GPU threads, ensuring efficient utilization of memory and compute bandwidth.

The experimental pipeline was designed to scale horizontally, making it adaptable for cloud-based or HPC cluster deployments. All shell-based generation scripts were structured to log resource consumption (VRAM, wall-clock time) and failure modes independently for each process.

The parallel execution framework is available in the repository and is based on the open-source utility \texttt{GNU Parallel} \cite{tange_2025_14911163}. We recommend citing this software when using the generation engine.

\begin{figure*}[ht]
    \centering
    \includegraphics[width=0.85\textwidth]{figures/diabetes/prompt_time_comparison.png}
    \caption{Generation Time Comparison for each Prompt}
    \label{fig:computation}
\end{figure*}

\begin{figure*}[ht]
    \centering
    \includegraphics[width=0.85\textwidth]{figures/stroke/generation_time_comparison.png}
    \caption{Generation Time Comparison for each model}
    \label{fig:computation-models}
\end{figure*}

\subsection*{Prompt Engineering Template}
For consistency in generation, all models were queried using structured prompt templates. An example template used in the diabetes dataset is as follows:

\begin{quote}
\texttt{Generate a synthetic patient record with the following fields: Age, Gender, BMI, Glucose Level, Blood Pressure, Diagnosis, and Treatment Recommendation. Ensure values are medically plausible.}
\end{quote}

The prompt was adapted based on model tokenization and output behavior. Post-processing scripts were applied to convert raw text responses into structured rows.

\subsection*{Synthetic Output Example}
Below is an example output from the Mistral model, after formatting:

\begin{quote}
\texttt{\{
  "gender": "Male",
  "age": 54,
  "hypertension": "Yes" or 1,
  "heart disease": "No" or 0,
  "smoking history": "never",
  "bmi": 31.4,
  "HbA1c level": 6.2,
  "blood glucose level": 178,
  "diabetes": "Yes" or 1
\}}
\end{quote}

This record passed all statistical and clinical validation checks.

\subsection*{Hyperparameter Summary}
\begin{table}[H]
\centering
\caption{Key hyperparameters for LLM fine-tuning and generation}
\begin{tabular}{|l|c|c|c|}
\hline
\textbf{Parameter} & \textbf{GPT} & \textbf{LLaMA} & \textbf{Mistral} \\
\hline
Max Tokens & 512 & 512 & 512 \\
Temperature & 0.7 & 0.6 & 0.5 \\
Top-p & 0.9 & 0.95 & 0.9 \\
LoRA Rank & N/A & 16 & 16 \\
Batch Size & 4 & 8 & 8 \\
Quantization & 8-bit & 4-bit & 4-bit \\
Inference Time (s/sample) & 1.8 & 1.1 & 0.9 \\
\hline
\end{tabular}
\end{table}

\subsection*{Metric Definitions}

To evaluate the quality of synthetic medical data comprehensively, we selected a diverse set of metrics drawn from statistics, machine learning, information theory, and privacy research. Each metric serves a specific evaluative goal: distributional alignment, structural consistency, medical plausibility, or privacy protection. Distributional metrics such as Wasserstein Distance and Kolmogorov-Smirnov help quantify how well synthetic data mirrors real data distributions. Structural metrics like Mutual Information and Silhouette Score evaluate dependencies and latent clustering. Privacy-related measures such as k-anonymity violation rates and adversarial accuracy detect potential disclosure risks. Together, this multi-perspective evaluation ensures a robust and holistic understanding of synthetic data fidelity and utility.

To supplement the quality assessment section, we define our core metrics:

\textbf{Wasserstein Distance (WD):} Measures the minimum cost required to morph one probability distribution into another \cite{villani2009optimal}. It accounts for the magnitude of differences in values, making it especially suitable for continuous numeric variables.

\textbf{Kolmogorov-Smirnov Statistic (KS):} Quantifies the maximum absolute difference between the cumulative distribution functions (CDFs) of two samples \cite{massey1951kolmogorov}. It is a non-parametric test often used for validating distributional similarity.

\textbf{Anderson-Darling k-Sample Test (AD):} A generalization of the KS test that compares the entire distributions of multiple samples, placing more weight on the tails \cite{scholz1987k}.

\textbf{Jensen-Shannon Divergence (JSD):} A symmetric variant of Kullback-Leibler divergence that measures the similarity between two probability distributions \cite{lin1991divergence}.

\textbf{Entropy Difference (H):} Measures the change in uncertainty between real and synthetic distributions \cite{shannon1948mathematical}. Significant entropy differences may indicate information loss or artificial patterns.

\textbf{Mutual Information Score (MI):} Quantifies the degree of dependency between features \cite{cover2012elements}. High mutual information indicates strong shared structure.

\textbf{Silhouette Score (SS):} Evaluates the cohesion and separation of clusters \cite{rousseeuw1987silhouettes}. Used to measure clustering quality after dimensionality reduction.

\textbf{k-Anonymity Violation Rate:} Proportion of synthetic samples that are distinguishable from fewer than \textit{k} real data points \cite{sweeney2002k}.

\textbf{Mahalanobis Anomaly Index (MAI):} Computes the distance of synthetic records from the mean of real data using the covariance matrix \cite{mahalanobis1936generalized}. High scores suggest potential anomalies.

\textbf{Medical Consistency Score (MCS):} Proportion of synthetic records adhering to rule-based validators for clinical logic.

\textbf{Nearest Neighbor Adversarial Accuracy (NNAA):} Evaluates distinguishability between real and synthetic samples using k-NN classifiers \cite{yale2020generation}. A score near 0.5 indicates good alignment.

This appendix aims to foster transparency and reproducibility, enabling independent verification and replication of our results.

\subsection*{Source Code and Reproducibility}
To facilitate reproducibility and further research, we have made the full SynLLM framework, including training scripts, prompt templates, evaluation utilities, and configuration files, publicly available on GitHub.

\begin{quote}
\textbf{GitHub Repository:} \url{https://github.com/ArshiaIlaty/SynLLM}
\end{quote}

Researchers and practitioners are encouraged to clone the repository, follow the provided setup instructions, and replicate experiments across supported hardware configurations. Contributions, issues, and extensions are welcomed via the GitHub issue tracker and pull requests.

\section{Implementation}

\subsection{Environment and Tooling}
The SynLLM framework is implemented in Python 3.10 using PyTorch as the underlying deep learning library. Model loading, fine-tuning, and inference tasks are facilitated through the Hugging Face Transformers library, while quantized loading and efficient inference are enabled using the BitsAndBytes package for 4-bit and 8-bit quantization. The experiments were conducted on a CUDA-enabled JupyterHub environment with access to three types of GPUs including, NVIDIA A100 with 80GB of VRAM (HBM2e), L40 8GB VRAM (GDDR6), and GTX 1080 Ti, each with 24 GB of VRAM, allowing efficient parallel model evaluation.

NVIDIA L40: 48GB VRAM (GDDR6)
NVIDIA A100: 80GB VRAM (HBM2e)
GTX 1080 Ti: 11GB VRAM (GDDR5X)

To streamline experimentation and ensure modularity, the codebase was organized into distinct modules for data preprocessing, model management, generation control, and evaluation. Version control and experiment tracking were handled using Git and manual logging to support reproducibility and collaboration.

\subsection{Model Configuration and Fine-Tuning}
Each selected LLM—GPT, LLaMA, and Mistral—was fine-tuned or prompt-engineered to align with structured medical data generation objectives. Tokenizers corresponding to each model were used to preserve compatibility with pre-trained embeddings. For Mistral and LLaMA, quantized 4-bit loading with LoRA (Low-Rank Adaptation) was employed to minimize memory overhead while preserving performance. Prompt templates were carefully crafted to reflect real-world patient records, including demographic fields, diagnostic labels, and laboratory results.

Model inference was conducted in batch mode, with deterministic decoding strategies (e.g., temperature=0, top\_p=0.9) to ensure repeatability. Each model generated a fixed number of synthetic samples per prompt, followed by parsing routines that transformed free-text outputs into structured tabular formats.

\subsection{Data Preprocessing and Management}
Datasets were standardized using min-max normalization for numerical features and one-hot encoding for categorical variables. Missing data imputation was handled using domain-informed median and mode values. The preprocessing pipeline also ensured the elimination of data leakage between training and evaluation phases by isolating synthetic generation from any real data statistics post-tokenization.

\subsection{Evaluation Pipeline}
The evaluation module was developed as a reusable Python class, incorporating functions for each metric category:
\begin{itemize}
    \item Statistical accuracy was assessed via pairwise KS tests, Wasserstein Distance, and histogram overlap metrics.
    \item Medical consistency was evaluated using predefined clinical validation rules, such as lab value thresholds, comorbidity co-occurrence logic, and expert-driven plausibility filters.
    \item Privacy risk was quantified using k-anonymity violation rates, record linkage analysis, and synthetic-to-real distance distributions.
    \item Anomaly detection was performed using Mahalanobis Distance and Local Outlier Factor (LOF) models trained on the real data distribution.
\end{itemize}
All metrics were logged and aggregated into visual summaries, including violin plots, density overlays, and correlation matrices, enabling intuitive comparison across models.

\subsection{Reproducibility and Experimental Rigor}
To ensure reproducibility, random seeds were fixed across all modules (NumPy, PyTorch, Transformers) and multiple experimental runs were conducted for each model to account for stochastic variations. Each experiment was independently repeated three times, and reported metrics represent the mean values across these runs.

Our pipeline emphasizes both scientific transparency and practical feasibility, setting a foundation for benchmarking future synthetic data frameworks.
